# Supplementary material for: Multiview Learning of Weighted Majority Vote by Bregman Divergence Minimization
Source: arXiv:1805.10212 source file (2018-05-25)
Supplement: Supplementary file 1 [file appendix.tex]

\section{Mathematical Tools}\label{stylefiles}
